# Supplementary material for: Ultra-low noise quantum memory for quasi-deterministic single photons generated by Rydberg collective atomic excitations
Source: arXiv:2111.08598 ancillary file (2021-11-25)
Supplement: Supplementary file 1 [file SM_Raman_storage_of_Rydberg_Photons.pdf]

# Supplementary Material:
# Ultra-low noise quantum memory for quasi-deterministic single photons generated by Rydberg collective atomic excitations

L. Heller,[1] J. Lowinski,[1] K. Theophilo,[1] A. Padrón-Brito,[1] and H. de Riedmatten[1,2]

[1]*ICFO - Institut de Ciencies Fotoniques, The Barcelona Institute of Science and Technology, Castelldefels (Barcelona) 08860, Spain*

[2]*ICREA-Institució Catalana de Recerca i Estudis Avançats, 08015 Barcelona, Spain*

## I. ESTIMATION OF $\mu_1$ PARAMETER (WITH SINGLE PHOTON INPUT)

An important figure of merit for a quantum memory is the parameter $\mu_1$, which is defined as the minimum mean number of input photons to have a signal-to-noise ratio (SNR) of 1 for the stored photon.

In Fig. 1 we show a measurement of SNR in the read-out (stored) detection window by varying the mean number of single photons at the input of the Raman memory. This is achieved by varying the Rydberg probe power (see Fig.2 of the main text). From a linear fit that passes through zero, we estimate a $\mu_1$ parameter of $1.00(7) \times 10^{-3}$.

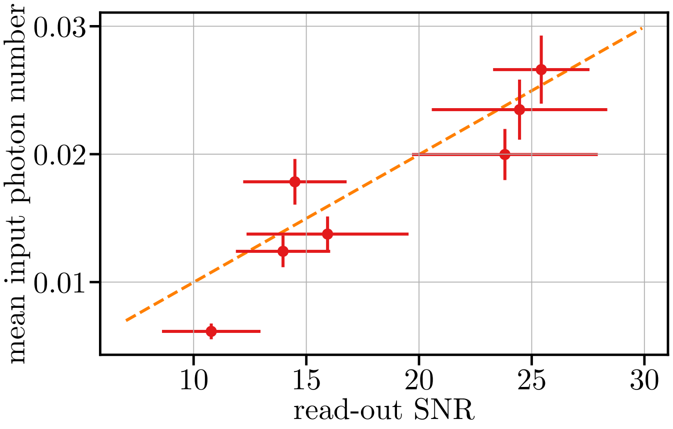


FIG. 1. Mean number of single photons at the input of the memory as a function of the read-out SNR. Orange dashed line: linear fit that passes through zero. The slope of this line corresponds to $\mu_1$.

## II. ACCEPTANCE MEMORY BANDWIDTH (WITH WEAK COHERENT STATES)

To understand whether the memory efficiency is limited by its acceptance bandwidth, we measure the storage and retrieval efficiency for input pulses with variable duration. The maximum duration of the single photons generated at the source is limited by the dephasing rate of the collective Rydberg excitations. Moreover, the minimum duration is limited by the coupling beam power, leading to FWHM greater than ∼90 ns. Therefore, we instead send weak coherent state (WCS) pulses with mean number of photons well below 1. The duration of the WCS pulses is controlled by an acousto-optic modulator (AOM), achieving pulses as short as 8 ns (FWHM). We send Gaussian-shaped pulses, because the conversion to bandwidth is straightforward.

The results are shown in Fig. 2. For pulse durations between 25 ns and 750 ns, the total efficiency $\eta_{wr}$ remains constant and is in agreement with the efficiencies measured for the single-photon input. Only for pulse durations below 25 ns, corresponding to a bandwidth of about ≈17.6 MHz (assuming transform-limited Gaussian pulses), the storage and retrieval efficiency drops. We attribute this drop to limited control power and finite AOM rise time, resulting in a smaller pulse area. For input pulses much longer than 750 ns (not characterised here), the efficiency is expected to be eventually limited by the lifetime of the memory [1]. We estimate the bandwidth of the single photon to be approximately 4 MHz, assuming bandwidth-limited Gaussian pulses.

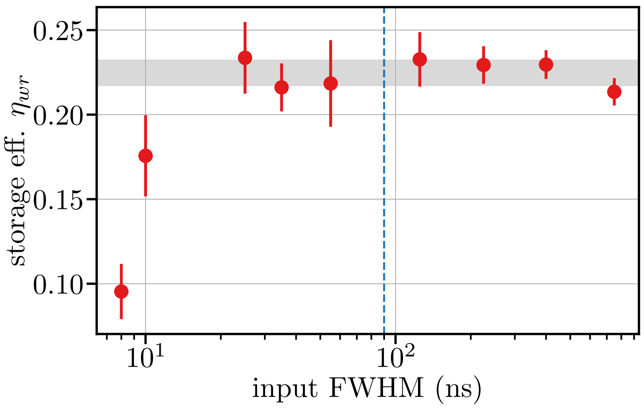


FIG. 2. Storage and retrieval efficiency $\eta_{wr}$ as a function of the temporal duration (FWHM) of WCS input pulses with Gaussian shape. Grey horizontal shaded area represents the mean (0.225) and standard deviation (0.008) of the efficiency for input pulse durations above 25 ns. Blue dashed vertical line represents the minimum duration of the single photon generated by the Rydberg-based source ( ∼90 ns FWHM). For each data point, write-in control pulse power, shape and delay are optimized.

## III. MEMORY PERFORMANCE WITH OPTICAL DEPTH (WITH WEAK COHERENT STATES)

It is instructive to analyse the memory performance when varying optical depth (OD), since OD governs how efficiently the incoming light pulse is absorbed and re-emitted. For that, we vary the trapping laser power during the magneto-optical trap stage and used the shortest interrogation time possible to be able to scan the full range of OD available.

The OD value is obtained by measuring the transmission of a continuous coherent beam around resonance with the $|g_s\rangle \to |e_s\rangle$ transition. Results are shown in Fig. 3. The storage efficiencies are measured for WCS pulses as input, shaped to mimic the temporal profile of the single photons generated in the Rydberg-based source.

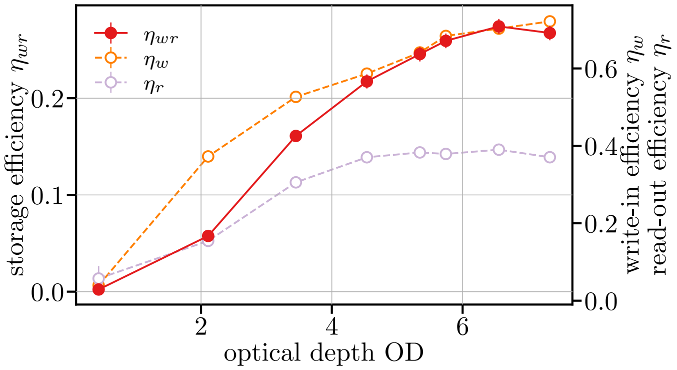


FIG. 3. Storage efficiencies $\eta_w$, $\eta_r$ and $\eta_{wr}$ as a function of the optical depth of the ensemble for weak coherent input pulses with a mean photon number of 0.077. For each data point, the write-in control pulse power and the delay are optimized.

We observe a saturation of the storage and retrieval efficiency $\eta_{wr} = \eta_w \cdot \eta_r$ for OD around 6.5. However, the write-in efficiency $\eta_w$ seems to still profit from higher OD, while read-out efficiency $\eta_r$ is already at the maximum. One possible explanation for this behaviour is re-emission followed by re-absorption, which limits the maximal retrieval efficiency in forward retrieval (i.e. when the photon field is retrieved from the medium co-propagating to the input) [2, 3].

Data in the main text was taken for OD around 5, which constitutes a compromise between achieving high $\eta_{wr}$ while at the same time maintaining an acceptable duty cycle for data acquisition.

## IV. EFFECT OF THE NOISE IN THE MEASURED AUTOCORRELATION FUNCTION OF SINGLE PHOTONS

Noise originated either from the control beam or its interaction with the ensemble can lead to uncorrelated coincidences that affect the measured single-photon statistics of the transmitted or stored photon. In the absence of control field and atoms, the unperturbed autocorrelation is measured as:

$$g^{(2)}_{\text{in}}(0) = \frac{c_{1,2}}{p_1 p_2}, \tag{1}$$

where $p_1$ ($p_2$) is the probability of detection per trial on detector 1(2), and $c_{1,2}$ is the probability of coincidence detection per trial between both detectors. When a storage attempt is performed, the noise introduced by the control pulses and the atoms alter the probabilities for detection and coincidences as follow:

$$\tilde{c}_{1,2} = c_{1,2} + p_1 p_{n,2} + p_2 p_{n,1} + p_{n,1} p_{n,2} \tag{2}$$

$$\tilde{p}_{1(2)} = p_{1(2)} + p_{n,1(2)}. \tag{3}$$

Here, $p_{n,1}$ ($p_{n,2}$) is the noise probability for detector 1(2). The autocorrelation is therefore:

$$\begin{aligned} g^{(2)}_{\text{out}}(0) &= \frac{\tilde{c}_{1,2}}{\tilde{p}_1 \tilde{p}_2} \\ &= \frac{p_{12} + p_1 p_{n,2} + p_2 p_{n,1} + p_{n,1} p_{n,2}}{p_1 p_2 + p_{n,1} p_2 + p_{n,2} p_1 + p_{n,1} p_{n,2}}, \end{aligned} \tag{4}$$

which can be rewritten in terms of SNRs as

$$g^{(2)}_{\text{out}}(0) = \frac{g^{(2)}_{\text{in}}(0) + 1/\text{SNR}_1 + 1/\text{SNR}_2 + 1/(\text{SNR}_1\text{SNR}_2)}{1 + 1/\text{SNR}_1 + 1/\text{SNR}_2 + 1/(\text{SNR}_1\text{SNR}_2)}, \tag{5}$$

where $\text{SNR}_{1(2)} = p_{1(2)}/p_{n,1(2)}$ is the signal-to-noise ratio for detector 1(2).

Assuming that SNR is the same for both detectors, this expression finally simplifies to

$$g^{(2)}_{\text{out}}(0) = \frac{g^{(2)}_{\text{in}}(0) + 2/\text{SNR} + 1/\text{SNR}^2}{1 + 2/\text{SNR} + 1/\text{SNR}^2}. \tag{6}$$

In Fig. 4, we characterize the effect of noise on the $g^{(2)}(0)$ of the stored and the transmitted photons for different values of $g^{(2)}(0)$ of the input photon (i.e. with no storage attempt). The input $g^{(2)}(0)$ was scanned by varying the mean number of photons in the probe (see Fig. 2 in the main text). We can see that, in general, the output $g^{(2)}(0)$ degrades compared to the input $g^{(2)}(0)$ and that the autocorrelation of the transmitted photon is better than the one of the stored photon. Therefore, we can conclude that the model qualitatively reproduces the expected trend. We attribute the imperfection in the quantitative analysis to low statistics and experimental fluctuations.

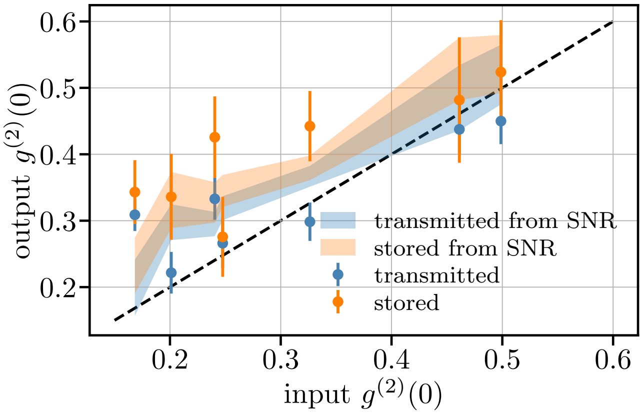


FIG. 4. Output $g^{(2)}(0)$ of the transmitted and the stored photons as a function of the input $g^{(2)}(0)$. Dashed black line: autocorrelation after the memory equals input. Shaded areas: autocorrelation for transmitted and stored photon as expected from eq. 6, taking into account uncertainty in $g^{(2)}_{\mathrm{in}}(0)$ and SNR.


[1] P. Farrera, G. Heinze, B. Albrecht, M. Ho, M. Chávez, C. Teo, N. Sangouard, and H. de Riedmatten, Generation of single photons with highly tunable wave shape from a cold atomic ensemble, Nature Communications **7**, 13556 (2016).

[2] K. F. Reim, J. Nunn, V. O. Lorenz, B. J. Sussman, K. C. Lee, N. K. Langford, D. Jaksch, and I. A. Walmsley, Towards high-speed optical quantum memories, Nat Photon **4**, 218 (2010), 10.1038/nphoton.2010.30.

[3] A. V. Gorshkov, A. Andre, M. Fleischhauer, A. S. Sørensen, and M. D. Lukin, Universal approach to optimal photon storage in atomic media, Physical Review Letters **98**, 123601 (2007).
